# Supplementary material for: Optimized Algorithms to Sample Determinantal Point Processes
Source: arXiv:1802.08471 source file (2018-02-23)
Supplement: Supplementary file 1 [file appendix.tex]

% !TEX root = ../main.tex

% ====================================================
% APPENDICES
% ====================================================
\ifels
\appendix 
\else
\appendix  \titleformat{\section}[hang]{\color{blue1}\large\bfseries\centering}{Appendix \thesection}{0mm}{}[]
\fi

% ===========================================
%
% ===========================================
\section{ \ifels\else - \fi Proof of Theorem~\ref{thm:main}}
\label{app:proof_thm_main}

\begin{proof}
	The theorem consists in proving that Eq.~\eqref{eq:coresets} is true. We follow a classical proof scheme from compressed sensing~\cite{baraniuk_simple_2008}, in four steps:
	\begin{enumerate}
		\item we first use concentration arguments for a given $\theta\in\Theta$. 
		\item we then build an $\epsilon$-net paving the space of parameters. 
		\item via the union bound, we obtain the result for all $\theta$ in the $\epsilon$-net.
		\item via the Lipschitz property of $f$, we obtain the desired result for all $\theta\in\Theta$.
	\end{enumerate}
	
	\textbf{Step 1} (Concentration around $\theta\in\Theta$) For a given $\theta\in\Theta$, we have the following concentration result~\cite{pemantle_concentration_2014}: $\forall\epsilon\in(0,1),  \forall\delta\in(0,1)$:
	\begin{align}
	\mathbb{P}\left(\left|\frac{\hat{L}}{L}-1\right|\geq\epsilon\right) = \mathbb{P}\left(\left|\hat{L}-L\right|\geq\epsilon L\right)\leq\delta,
	\end{align}
	provided that:
	\begin{align}
	\label{eq:to_replace_if_mDPP}
	\mu\geq \frac{16}{\epsilon^2} \left(\epsilon C + 2 C^2\right) \log{\frac{5}{\delta}},
	\end{align}
	with $C=\displaystyle \max_{i} \frac{f(x_i, \theta)}{L\bar{\pi}_i}.$ 
	
	Using the same concentration results, we also have:
	\begin{align}
	\label{eq:conc_size}
	\forall(\epsilon,\delta)\in(0,1)^2,~~\mathbb{P}\left(\left|\frac{\sum_{i}\frac{\epsilon_i}{\pi_i}}{N}-1\right|\geq\epsilon\right) \leq\delta,
	\end{align}
	provided that:
	\begin{align}
	\label{eq:to_replace_if_mDPP}
	\mu\geq \frac{16}{\epsilon^2N\bar{\pi}_{\text{min}}} \left(\epsilon + \frac{2}{N\bar{\pi}_{\text{min}}}\right) \log{\frac{5}{\delta}}.
	\end{align}
	
	\textbf{Step 2} ($\epsilon'$-net of $\Theta$) Consider $\Gamma_{\epsilon'} = (\theta^*_1,\ldots,\theta^*_{n_{\epsilon'}})$ the smallest subset of $\Theta$ such that balls of radius $\epsilon'$ centered around the elements in $\Gamma_{\epsilon'}$ cover $\Theta$. $\Gamma_{\epsilon'}$ is called an $\epsilon'$-net of $\Theta$ and $n_{\epsilon'}$ its covering number. The covering property entails that:
	\begin{align}
	\forall\theta\in\Theta\quad\exists\theta^*\in\Gamma_{\epsilon'}~~~\text{ s.t. }~~~d_\Theta(\theta,\theta^*)\leq\epsilon'.
	\end{align}
	
	\textbf{Step 3.} (Union bound) 
	Write $\delta' = \delta / 2n_{\epsilon'}$. 
	From step 1, we know that, $\forall\theta^*\in\Gamma_{\epsilon'}$:
	\begin{align}
	\mathbb{P}\left(\left|\frac{\hat{L}}{L}-1\right|\geq\epsilon\right) \leq\delta'
	\end{align}
	provided that:
	\begin{align}
	\mu\geq \frac{16}{\epsilon^2} \left(\epsilon C + 2 C^2\right) \log{\frac{5}{\delta'}}.
	\end{align}
	From the union bound, we have:
	\begin{align}
	\mathbb{P}\left(\forall\theta^*\in\Gamma_{\epsilon'},\quad \left|\frac{\hat{L}}{L}-1\right|\leq \epsilon\right)\geq 1-\sum_{\theta^*\in\Gamma}\delta' = 1-\frac{\delta}{2},
	\end{align}
	provided that:
	\begin{align}
	\label{eq:pre_condition}
	\mu\geq \frac{16}{\epsilon^2} \max_{\theta^*\in\Gamma_{\epsilon'}}\left(\epsilon C + 2 C^2\right) \log{\frac{10n_{\epsilon'}}{\delta}}.
	\end{align}
	Given that $\bar{\pi}_i$ will \textit{in fine} be independent of $\theta$ (as we want the coreset property to be true for all $\theta\in\Theta$),
	\begin{align}
	\max_{\theta^*\in\Gamma_{\epsilon'}} C &= \max_{\theta^*\in\Gamma_{\epsilon'}}\max_{i} \frac{f(x_i, \theta)}{L\bar{\pi}_i}\\
	&=\max_{i} \frac{1}{\bar{\pi}_i}\max_{\theta^*\in\Gamma_{\epsilon'}}\frac{f(x_i, \theta)}{L}\\
	&\leq \max_{i} \frac{1}{\bar{\pi}_i} \max_{\theta\in\Theta}\frac{f(x_i, \theta)}{L} = \max_{i} \frac{\sigma_i}{\bar{\pi}_i}
	\end{align}
	such that Eq.~\eqref{eq:pre_condition} is verified if $\mu\geq \mu_1$ with
	\begin{align}
	\mu_1 = \frac{16}{\epsilon^2} \left(\epsilon \max_{i} \frac{\sigma_i}{\bar{\pi}_i} + 2 \left(\max_{i} \frac{\sigma_i}{\bar{\pi}_i}\right)^2 \right) \log{\frac{10n_{\epsilon'}}{\delta}}.
	\end{align}

	Write $\delta'' = \delta / 2$. From Eq.~\eqref{eq:conc_size}, we have:
	\begin{align}
	\mathbb{P}\left(\left|\frac{\sum_{i}\frac{\epsilon_i}{\pi_i}}{N}-1\right|\geq\epsilon\right) \leq\delta'',
	\end{align}
	provided that $\mu\geq \mu_2$ with
	\begin{align}
	\mu_2=\frac{16}{\epsilon^2N\bar{\pi}_{\text{min}}} \left(\epsilon + \frac{2}{N\bar{\pi}_{\text{min}}}\right) \log{\frac{10}{\delta}}.
	\end{align}
	We have (with the union bound again):
	\begin{align}
	\mathbb{P}&\left( \left|\frac{\sum_{i}\frac{\epsilon_i}{\pi_i}}{N}-1\right|\leq\epsilon \quad \text{AND} \quad \forall\theta^*\in\Gamma_{\epsilon'},\quad \left|\frac{\hat{L}}{L}-1\right|\leq \epsilon\right)\nonumber\\
	&\qquad\qquad\qquad\geq 1-\delta/2-\delta'' = 1-\delta,
	\end{align}
	provided that:
	\begin{align}
	\mu\geq \max (\mu_1, \mu_2).
	\end{align}
	
	\textbf{Step 4} (Continuity argument) 
	Define 
	
	Suppose that $\mu\geq \max (\mu^*_1, \mu^*_2)$. The result of step 3 with $\epsilon \leftarrow \epsilon/2$ states that, with probability at least $1-\delta$, one has:
	\begin{align}
	\label{eq:concentration_eps_net}
	\left|\frac{\sum_{i}\frac{\epsilon_i}{\pi_i}}{N}-1\right|\leq\frac{\epsilon}{2}\quad\text{AND}\quad\forall\theta^*\in\Gamma_{\epsilon'}, ~~\left|\frac{\hat{L}}{L}-1\right|\leq \frac{\epsilon}{2}.
	\end{align}
	
	We now look for the maximum value of $\epsilon'$ such that Eq.~\eqref{eq:concentration_eps_net} implies the following desired result:
	\begin{align}
	\label{eq:desired_result}
	\forall\theta\in\Theta, \qquad\left|\frac{\hat{L}}{L}-1\right|\leq \epsilon.
	\end{align}
	
	Consider $\theta\in\Theta$. By the covering property of $\Gamma_{\epsilon'}$, we have:
	\begin{align}
	\exists\theta^*\in\Gamma_{\epsilon'} ~\text{ s.t. } ~d_\Theta(\theta,\theta^*)\leq\epsilon'.
	\end{align}
	Moreover, as $f$ is $\gamma$-Lipschitz, $\forall x_i\in\mathcal{X}$:
	\begin{align}
	\label{eq:Lipschitz}
	|f(x_i,\theta)-f(x_i,\theta^*)|\leq \gamma ~d_\Theta(\theta,\theta^*)\leq \gamma \epsilon'.
	\end{align}
	Thus, using Eqs.~\eqref{eq:concentration_eps_net} and~\eqref{eq:Lipschitz}:
	\begin{align}
	\hat{L}(\mathcal{X},\theta)&\leq \hat{L}(\mathcal{X},\theta^*) + \gamma\epsilon'\sum_i \frac{\epsilon_i}{\pi_i}\\
	&\leq (1+\frac{\epsilon}{2})(L(\mathcal{X},\theta^*) + N\gamma\epsilon').
	\end{align}
	Also, using Eq.~\eqref{eq:Lipschitz} again:
	\begin{align}
	L(\mathcal{X},\theta^*)\leq L(\mathcal{X},\theta) + N\gamma\epsilon'.
	\end{align}
	Thus:
	\begin{align}
	\label{eq:higher_bound}
	\hat{L}(\mathcal{X},\theta)&\leq (1+\frac{\epsilon}{2})L(\mathcal{X},\theta) + 2N\gamma\epsilon'(1+\frac{\epsilon}{2}).
	\end{align}
	Similarly, for the lower bound, one obtains:
	\begin{align}
	\label{eq:lower_bound}
	(1-\frac{\epsilon}{2})L(\mathcal{X},\theta) - 2N\gamma\epsilon'\leq \hat{L}(\mathcal{X},\theta)
	\end{align}
	In order for Eqs~\eqref{eq:higher_bound} and~\eqref{eq:lower_bound} to imply Eq.\eqref{eq:desired_result}, we need:
	\begin{align}
	2N\gamma\epsilon'(1+\frac{\epsilon}{2}) \leq \frac{\epsilon}{2}L(\mathcal{X},\theta),
	\end{align}
	\ie:
	\begin{align}
	\epsilon'\leq \frac{\epsilon L(\mathcal{X},\theta)}{4N\gamma(1+\frac{\epsilon}{2})}\leq \frac{\epsilon L(\mathcal{X},\theta)}{6N\gamma}.
	\end{align}
	In order for this condition to be true for all $\theta$, we choose:
	\begin{align}
	\label{eq:epsilonprime}
	\epsilon' = \frac{\epsilon\min_{\theta\in\Theta} L(\mathcal{X},\theta)}{6N\gamma} = \frac{\epsilon L^{\text{opt}}}{6N\gamma}=  \frac{\epsilon \langle f\rangle_\text{opt}}{6\gamma}.
	\end{align}
	
	\textbf{Concluding the proof.}
	Consider $\mathcal{S}$ a sample from a DPP with kernel $\ma{K}$, marginal probabilities of inclusion $\ma{K}_{ii} = \pi_i$ and normalized marginal probabilities $\bar{\pi}_i=\pi_i/\mu$.  Consider $\epsilon\in(0,1)$ and $\delta\in(0,1)$. Define $\epsilon'$ as in Eq.~\eqref{eq:epsilonprime} and $\Gamma$ the set of centers of the $n_{\epsilon'}$ balls of radius $\epsilon'$ covering the parameter space. We showed that if $\mu\geq \max (\mu^*_1, \mu^*_2)$, then $\mathcal{S}$ is an $\epsilon$-coreset with probability at least $1-\delta$. 
\end{proof}

\section{ \ifels\else - \fi Proof of two Lemmas}
\label{app:proof_lemmas}

\begin{lemma}
	In the $1$-means problem (the $k$-means problem with $k=1$), and supposing without loss of generality that the data is centered (\ie: $\sum_j x_j = 0$), we have:
	\begin{align}
	\sigma_i = \frac{1}{N}\left(1+\frac{\norm{x_i}^2}{v}\right),
	\end{align}
	where $v=\frac{1}{N}\sum_{x\in\mathcal{X}} \norm{x}^2$.
\end{lemma}

\begin{proof}
	By definition: 
	$$\frac{1}{\sigma_i}=\min_{c} \frac{\sum_x \norm{x-c}^2}{\norm{x_i-c}^2}.$$
	Consider $\mathcal{S}(x_i,R)$ the sphere centered on $x_i$ and radius $R\geq0$. We have that:
	\begin{align*}
	\min_{c} ~~ = ~~~~\min_{R\geq 0 } ~~~\min_{c\in\mathcal{S}}
	\end{align*}
	We thus have:
	\begin{align*}
	\frac{1}{\sigma_i}=\min_{R\geq 0 } \frac{1}{R^2}  \min_{c\in\mathcal{S}}  \sum_x \norm{x-c}^2.
	\end{align*}
	Writing $x-c= x - x_i - (c-x_i)$, we may write 
	\begin{align*}
	\sum_{x}\norm{x - c}^2 = NR^2 + &\sum_{x}\norm{x - x_i}^2  \\
	&- 2R \norm{\sum_{x} x - x_i} \cos{\theta},
	\end{align*}
	with $\theta$ the angle formed by $\sum_{x} x - x_i$ and $c - x_i$. As the minimum is seeked for $c$ on the sphere, the angle $\theta$ may take any value, such that the minimum is always attained with $\theta$ s.t. $\cos{\theta}=1$. We finally obtain:
	\begin{align*}
	\frac{1}{\sigma_i}=N+\min_{R\geq 0 } \frac{1}{R^2}  \left(\sum_{x}\norm{x - x_i}^2  - 2R \norm{\sum_{x} x - x_i} \right).
	\end{align*} 
	Studying analytically the function $f(R) = \frac{a-2bR}{R^2}$, its minimum is attained for $R^* = \frac{a}{b}$ and $f(R^*) = -\frac{b^2}{a}$, such that:
	\begin{align*}
	\frac{1}{\sigma_i} 
	=  N - \frac{||\sum_{x} x-x_i||^2}{\sum_{x}\norm{x-x_i}^2}.
	\end{align*}
	Supposing without loss of generality that the data is centered, \ie: $\sum_x x = 0$ and denoting $v=\frac{1}{N}\sum_x \norm{x}^2$, we have:
	\begin{align*}
	\frac{1}{\sigma_i} 
	=  N - \frac{N^2\norm{x_i}^2}{Nv + N\norm{x_i}^2}.
	\end{align*}
	Inverting this equation yields:
	\begin{align*}
	\sigma_i 
	&= \frac{v+\norm{x_i}^2}{Nv+N\norm{x_i}^2 - N \norm{x_i}^2}\\
	&= \frac{1}{N}\left(1+\frac{\norm{x_i}^2}{v}\right)
	\end{align*}
\end{proof}

\begin{lemma}
	In the $k$-means problem, $N\sigma_{\text{min}}\geq 1$.
\end{lemma}

\begin{proof}
	Consider $\theta^\text{opt}=(c_1^\text{opt}, \ldots, c_k^\text{opt})$ the optimal solution of $k$-means and $\{\mathcal{V}_1, \mathcal{V}_2, \ldots, \mathcal{V}_k\}$ their associated Voronoi sets. Consider $x_i\in\mathcal{X}$ and suppose, without loss of generality that $x_i\in\mathcal{V}_1$. Also, for any $x\in\mathcal{X}$, we denote by $c(x) = \argmin_{c\in\theta} \norm{x-c}^2$. We have:
	\begin{align*}
	\frac{1}{\sigma_i} &= \min_{c_1, \ldots, c_k} \frac{\sum_{x\in\mathcal{X}} \norm{x - c(x)}^2}{\norm{x_i - c(x_i)}^2}\\
	&=\min_{c_1, \ldots, c_k} \frac{\sum_{x\in\mathcal{V}_1} \norm{x - c(x)}^2}{\norm{x_i - c(x_i)}^2} + \sum_{j=2}^k \frac{\sum_{x\in\mathcal{V}_j} \norm{x - c(x)}^2}{\norm{x_i - c(x_i)}^2}
	\end{align*}
	Given that, by definition of $c(x)$, $\forall j, ~\norm{x-c(x)}^2 \leq \norm{x-c_j}^2$, we have:
	\begin{align*}
	\frac{1}{\sigma_i} 
	\leq \min_{c_1, \ldots, c_k} \frac{\sum_{x\in\mathcal{V}_1} \norm{x - c_1}^2}{\norm{x_i - c(x_i)}^2} + \sum_{j=2}^k \frac{\sum_{x\in\mathcal{V}_j} \norm{x - c_j}^2}{\norm{x_i - c(x_i)}^2}
	\end{align*}
	To further bound this quantity, let us constrain the domain over which the minimum is seeked.  Consider $\mathcal{B}(x_i,R)$ the ball centered on $x_i$ and radius $R\geq0$. Consider $\mathcal{S}(x_i,R)$ its surface (\ie, the associated sphere). We have that:
	\begin{align*}
	\min_{c_1, \ldots, c_k} ~~\leq ~~~~\min_{R\geq 0 } ~~~\min_{c_1\in\mathcal{S}, (c_2,\ldots, c_k)\notin\mathcal{B}}
	\end{align*}
	Given this restricted search space, we have: $c(x_i) = c_1$ and $\norm{x_i - c_1}^2 = R^2$, and thus:
	\begin{align*}
	\frac{1}{\sigma_i} 
	~~\leq~~ &\min_{R\geq 0 } \frac{1}{R^2}  \min_{c_1\in\mathcal{S}} \left(\sum_{x\in\mathcal{V}_1} \norm{x - c_1}^2  \right.\\
	&\left.+ \min_{(c_2,\ldots, c_k)\notin\mathcal{B}} \sum_{j=2}^k \sum_{x\in\mathcal{V}_j} \norm{x - c_j}^2\right)
	\end{align*}
	Now, one may show, for all $j=2, \ldots, k$, that:
	\begin{align*}
	\sum_{x\in\mathcal{V}_j} \norm{x - c_j}^2 = \sum_{x\in\mathcal{V}_j} \norm{x - c_j^\text{opt}}^2 + \#\mathcal{V}_j \norm{c_j-c_j^\text{opt}}^2,
	\end{align*}
	due to the fact that $c_j^\text{opt} = \frac{1}{\#\mathcal{V}_j} \sum_{x\in\mathcal{V}_j}  x$. 
	Given that the minimum of $\norm{c_j-c_j^\text{opt}}^2$ is necessarily smaller than $R^2$:
	\begin{align*}
	\min_{c_j\notin\mathcal{B}}	\sum_{x\in\mathcal{V}_j} \norm{x - c_j}^2 \leq \sum_{x\in\mathcal{V}_j} \norm{x - c_j^\text{opt}}^2 + \#\mathcal{V}_j R^2, 
	\end{align*}
	such that:
	\begin{align*}
	\frac{1}{\sigma_i} 
	\leq &  \min_{R\geq 0 } \frac{1}{R^2} 
	\min_{c_1\in\mathcal{S}} \left(\sum_{x\in\mathcal{V}_1} \norm{x - c_1}^2  
	+ \alpha + (N-\#\mathcal{V}_1)R^2\right)\\
	&=N-\#\mathcal{V}_1 + \min_{R\geq 0 } \frac{1}{R^2} \min_{c_1\in\mathcal{S}}  \left(\sum_{x\in\mathcal{V}_1} \norm{x - c_1}^2  
	+ \alpha\right)
	\end{align*}
	with $\alpha = L^{\text{opt}\backslash\mathcal{V}}$ the optimal $(k-1)$-means cost on $\mathcal{X}\backslash\mathcal{V}$.  
	Writing $x-c_1= x - x_i - (c_1-x_i)$, we may decompose $
	\sum_{x\in\mathcal{V}_1}\norm{x - c_1}^2$ in $R^2\#\mathcal{V}_1 + \sum_{x\in\mathcal{V}_1}\norm{x - x_i}^2  - 2R \norm{\sum_{x\in\mathcal{V}_1} x - x_i} \cos{\theta}$, 
	with $\theta$ the angle formed by $\sum_{x\in\mathcal{V}_1} x - x_i$ and $c_1 - x_i$. As the minimum is seeked for $c_1$ on the sphere, the angle $\theta$ may take any value, such that the minimum is always attained with $\theta$ s.t. $\cos{\theta}=1$. We finally obtain, denoting $\forall x\in\mathcal{V}_1,~y = x-x_i$:
	\begin{align*}
	\frac{1}{\sigma_i} 
	\leq &  N + \min_{R\geq 0 } \frac{1}{R^2} \left(\sum_{x\in\mathcal{V}_1}\norm{y}^2  - 2R \norm{\sum_{x\in\mathcal{V}_1} y} + \alpha\right). 
	\end{align*}
	Studying analytically the function $f(R) = \frac{a-2bR+\alpha}{R^2}$, its minimum is attained for $R^* = \frac{a+\alpha}{b}$ and $f(R^*) = -\frac{b^2}{a+\alpha}$, such that:
	\begin{align*}
	\frac{1}{\sigma_i} 
	\leq &  N - \frac{||\sum_{x\in\mathcal{V}_1} y||^2}{\sum_{x\in\mathcal{V}_1}\norm{y}^2 + \alpha} \leq N.
	\end{align*}
	This is true for all $i$, and in particular for $\sigma_{\text{min}}$. 
\end{proof}

\section{ \ifels\else - \fi Proofs concerning the DPP sampling algorithms}
\label{app:proofs_sampling}

\begin{lemma}
Supposing that $\ma{K}$ is a projective matrix, that is: $\ma{K}=\Fou_\mathcal{J}\Fou_\mathcal{J}^\adjoint$ with $\Fou_\mathcal{J}^\adjoint\Fou_\mathcal{J}=\ma{I}_J$ the identity matrix of dimension $J$,  Alg.~\ref{alg:sampling_m-DPP} samples a DPP associated to kernel $\ma{K}$. The number of samples of the output is necessarily $J=|\mathcal{J}|$. 
\end{lemma}

\begin{proof}
	We denote by $\mathcal{S}$ the output of Alg.~\ref{alg:sampling_m-DPP}. Let us also denote by $\mathcal{S}_n$ (resp. $p_n(i)$) the sample set (resp. the value of $p(i)$) at the end of the $n$-th iteration of the loop of Alg.~\ref{alg:sampling_m-DPP}. We have : $\mathcal{S}_n = \mathcal{S}_{n-1}\cup\{s_n\}$. 
	Using the Schur complement, we have : 
	\begin{align}
	\label{eq:pn}
	\forall n\in[1,J]\;,\forall i\qquad\text{det}\left(\ma{K}_{\mathcal{S}_{n-1}\cup\{i\}}\right) &= \left(\ma{K}_{i,i} - \ma{K}_{\mathcal{S}_{n-1},i}^\adjoint\ma{K}_{\mathcal{S}_{n-1}}^{-1}\ma{K}_{\mathcal{S}_{n-1},i}\right) \;\text{det}\left(\ma{K}_{\mathcal{S}_{n-1}}\right) \nonumber\\
	& = p_{n-1}(i)\;\text{det}\left(\ma{K}_{\mathcal{S}_{n-1}}\right).
	\end{align}
	Given Eq.~\eqref{eq:pn}, and knowing that $\ma{K}$ is SDP: $\forall\mathcal{S}, \,\text{det}(\ma{K}_\mathcal{S})\geq0$, one can show that $p_n(i)\geq 0$ and $\sum_i{p_n}(i)\neq 0$: at each iteration $n$, the probability  $\mathbb{P}(s)=\frac{p_n(s)}{\sum_i p_n(i)}$ is well defined. 
	% 
	%ce qui implique %, vue l'équation~\eqref{eq:pn}, que 
	%$p_n(i)\geq 0$. De plus, $\sum_i{p_n}(i)\neq 0$. En effet, si ce n'était pas le cas, cela impliquerait $\forall i, p_n(i)=0$, \ie, d'après~\eqref{eq:pn}, 
	%$
	%\forall i, \quad\text{det}\left(\ma{K}_{\bar{\mathcal{S}}\cup\{i\}}\right)=0,
	%$
	%\ie, le rang de $\ma{K}$ serait inférieur à $m$, ce qui est  contraire à l'hypothèse.  \`A chaque itération de la boucle, la probabilité $\mathbb{P}(s)$ est donc bien définie.  
	The loop being repeated $J$ times, the number of samples of the output is thus necessarily equal to $J$. 
	
	Let us now show that $\mathbb{P}(\mathcal{S})$ is indeed of determinantal form. By construction of $\mathcal{S}$ :
		\begin{align}
		\mathbb{P}(\mathcal{S}) &= \prod_{l=1}^J \mathbb{P}(s_l|s_1, s_2,\ldots, s_{l-1})=\prod_{l=1}^J \frac{p_{l-1}(s_l)}{\sum_{i=1}^N p_{l-1}(i)}.\label{eq:prod_cond}
		\end{align}
		Writing Eq.~\eqref{eq:pn} for $i=s_n$, and iterating, one obtains  :
		$\prod_{l=1}^J p_{l-1}(s_l)=\text{det}(\ma{K}_{\mathcal{S}})$. 
		Let us finish by showing that the denominator of Eq~\eqref{eq:prod_cond} does not depend on the chosen samples. This is where the projective assumption of $\ma{K}$ is essential. One has :
		\begin{align}
		\forall l\in[1,m], \qquad \sum_{i=1}^N p_{l-1}(i) = \sum_{i=1}^N p_{0}(i) - \sum_{i=1}^N \ma{K}_{\mathcal{S}_{l-1},i}^\adjoint\ma{K}_{\mathcal{S}_{l-1}}^{-1}\ma{K}_{\mathcal{S}_{l-1},i}\nonumber
		\end{align}
		We have $\sum_{i=1}^N p_{0}(i)=\text{Tr}(\Fou_\mathcal{J}\Fou_\mathcal{J}^\adjoint)=\text{Tr}(\Fou_\mathcal{J}^\adjoint\Fou_\mathcal{J})=J$. Moreover, let us write $\ma{M}$ the measurement matrix associated to $\mathcal{S}_{l-1}$:
		\begin{align}
		\ma{M} = (\vec{\delta}_{s_1}|\ldots|\vec{\delta}_{s_{l-1}})^\adjoint\in\mathbb{R}^{l-1\times N}.
		\end{align}
		We have:
		\begin{align}
		\sum_{i=1}^N &\ma{K}_{\mathcal{S}_{l-1},i}^\adjoint\ma{K}_{\mathcal{S}_{l-1}}^{-1}\ma{K}_{\mathcal{S}_{l-1},i} = \text{Tr}\left(\Fou_\mathcal{J}\Fou_\mathcal{J}^\adjoint\ma{M}^\adjoint (\ma{M}\Fou_\mathcal{J}\Fou_\mathcal{J}^\adjoint\ma{M}^\adjoint)^{-1}\ma{M}\Fou_\mathcal{J}\Fou_\mathcal{J}^\adjoint\right)\nonumber\\
		&=\text{Tr}\left((\ma{M}\Fou_\mathcal{J}\Fou_\mathcal{J}^\adjoint\ma{M}^\adjoint)^{-1}\ma{M}\Fou_\mathcal{J}\Fou_\mathcal{J}^\adjoint\Fou_\mathcal{J}\Fou_\mathcal{J}^\adjoint\ma{M}^\adjoint \right) = \text{Tr}(\ma{I}_{l-1}) = l-1\nonumber,
		\end{align}
		by invariance of the trace by circular permutations. Thus :
		\begin{align}
		\mathbb{P}(\mathcal{S}) = \frac{1}{Z} \text{det}(\ma{K}_{\mathcal{S}}) \text{~with~} Z = \prod_{l=1}^J J-l+1=J\,!
		\end{align}
		which ends the proof.
\end{proof}

\begin{lemma}
	Assume that $\forall k\in\mathcal{J}$ $\vec{u}_k\in\mathbb{R^N}$ verifies the following low-dimensional representation:
	\begin{align}
	\vec{u}_k = \frac{1}{\sqrt{\nu_k}}\ma{\Psi}^\adjoint\vec{v}_k,
	\end{align}
	where $\vec{v}_k\in\mathbb{R}^{2r}$ are orthonormal, $\nu_k>0$, and $\ma{\Psi}\in\mathbb{R}^{2r\times N}$. Write $\ma{V}_\mathcal{J}\in\mathbb{R}^{2r\times J}$ the matrix concatenating all $\vec{v}_k$ such that $k\in\mathcal{J}$. Alg.~\ref{alg:sampling_m-DPP_dual} with inputs $\ma{V}_\mathcal{J}$, $\{\nu_k\}_{k\in\mathcal{J}}$ and $\ma{\Psi}$ is equivalent to Alg.~\ref{alg:sampling_m-DPP} with input $\Fou_\mathcal{J}$.
\end{lemma}

\begin{proof}
	The proof consists in showing a point-by-point equivalence in all the steps of the algorithms. Given the low-dimensional representation of $\vec{u}_k$ and denoting $\ma{D}_J=\text{diag}(\{\nu_k\}_{k\in\mathcal{J}})\in\mathbb{R}^{\mathcal{J}\times\mathcal{J}}$, we have:
	\begin{align}
		\ma{U}_J = \ma{\Psi}^\adjoint\ma{V}_\mathcal{J}\ma{D}_J^{-\frac{1}{2}}.
	\end{align}
	Defining $\tilde{\ma{U}}_J$ as in Alg.~\ref{alg:sampling_m-DPP_dual}:
	\begin{align}
		\tilde{\ma{U}}_J = \ma{V}_\mathcal{J}\ma{D}_J^{-\frac{1}{2}},
	\end{align}
	such that 
	\begin{align}
		\ma{U}_J = \ma{\Psi}^\adjoint\tilde{\ma{U}}_J.
	\end{align}
	Thus, the initial computation of $p_0(i)$ is equivalent:
	\begin{align}
		p_0(i) = \norm{\tilde{\ma{U}}_J^\adjoint\vec{\psi}_i}^2 = \norm{\tilde{\ma{U}}_J^\adjoint\ma{\Psi}\vec{\delta}_i}^2 = \norm{\ma{U}_J^\adjoint\vec{\delta}_i}^2.
	\end{align}
	We now show that, at each iteration $n$ of the loop:
	\begin{align}
		\forall i, \qquad	\ma{K}_{\mathcal{S},i}^\adjoint \ma{K}_{\mathcal{S}}^{-1} \ma{K}_{\mathcal{S},i} = \vec{\psi}_i^\adjoint \tilde{\ma{C}}_\mathcal{J} \ma{\Psi}_\mathcal{S}\tilde{\ma{C}}_\mathcal{S}^{-1} \ma{\Psi}_\mathcal{S}^\adjoint\tilde{\ma{C}}_\mathcal{J} \vec{\psi}_i,
	\end{align}
	where 
	\begin{align}
		\ma{K} = \ma{U}_J\ma{U}_J^\adjoint,
	\end{align}
	and
	\begin{align}
		\tilde{\ma{C}}_\mathcal{S}^{-1}=(\ma{\Psi}_\mathcal{S}^\adjoint\tilde{\ma{C}}_\mathcal{J}\ma{\Psi}_\mathcal{S})^{-1}\in\mathbb{R}^{n\times n} \quad\text{ with }\quad \tilde{\ma{C}}_\mathcal{J} = \tilde{\ma{U}}_\mathcal{J}\tilde{\ma{U}}_\mathcal{J}^\adjoint\in\mathbb{R}^{2r \times 2r}\quad\text{ and }\quad \ma{\Psi}_\mathcal{S}=(\vec{\psi}_{s_1}|\ldots|\vec{\psi}_{s_n}).
	\end{align}
	Indeed:
	\begin{align}
		\ma{\Psi}_\mathcal{S}^\adjoint\tilde{\ma{C}}_\mathcal{J}\ma{\Psi}_\mathcal{S} = (\vec{\delta}_1|\ldots|\vec{\delta}_{s_n})^\adjoint\Psi^\adjoint\tilde{\ma{U}}_\mathcal{J}\tilde{\ma{U}}_\mathcal{J}^\adjoint\Psi(\vec{\delta}_1|\ldots|\vec{\delta}_{s_n}) = \ma{K}_\mathcal{S},
	\end{align}
	such that $\tilde{\ma{C}}_\mathcal{S}^{-1} = \ma{K}_\mathcal{S}^{-1}$. Similarly, we show that $\ma{K}_{\mathcal{S},i} = \ma{\Psi}_\mathcal{S}^\adjoint\tilde{\ma{C}}_\mathcal{J} \vec{\psi}_i$, which ends the proof. 
\end{proof}	

\begin{lemma}
	Given the same low-dimensional assumptions as in the previous lemma, Alg.~\ref{alg:sampling_r-DPP_bis_dual_efficient} is equivalent to Alg.~\ref{alg:sampling_m-DPP_dual}.
\end{lemma}

\begin{proof}
	Let us denote by $\mathcal{S}_n$ (resp. $p_n(i)$) the sample set (resp. the value of $p(i)$) at the end of the $n$-th iteration of the loop. We have : $\mathcal{S}_n = \mathcal{S}_{n-1}\cup\{s_n\}$. All we need to show is that the $p_n(i)$ are equal in both algorithms. In Alg.~\ref{alg:sampling_r-DPP_bis_dual_efficient} : $p_n(i) = p_{n-1}(i) - (\vec{f}_n^\adjoint\vec{\psi}_i)^2 = p_0(i) - \sum_{l=1}^{n} (\vec{f}_l^\adjoint\vec{\psi}_i)^2$ (where the $\{\vec{f}_i\}$ are defined in the algorithm). Comparing with the  $p_n(i)$ of Alg.~\ref{alg:sampling_m-DPP_dual}, all we need to show is:
	\begin{align}
	\forall n\forall i \quad \quad
	\sum_{l=1}^{n} (\vec{f}_l^\adjoint\vec{\psi}_i)^2= \vec{\psi}_i^\adjoint\tilde{\ma{C}}_\mathcal{J} \ma{\Psi}_\mathcal{S}\tilde{\ma{C}}_\mathcal{S}^{-1} \ma{\Psi}_\mathcal{S}^\adjoint\tilde{\ma{C}}_\mathcal{J}\vec{\psi}_i.
	\end{align}
	We will show more generally that:
	\begin{align}
	\label{eq:to_proove}
	\forall n  \quad \quad
	\sum_{l=1}^{n} \vec{f}_l\vec{f}_l^\adjoint =  \tilde{\ma{C}}_\mathcal{J} \ma{\Psi}_\mathcal{S}\tilde{\ma{C}}_\mathcal{S}^{-1} \ma{\Psi}_\mathcal{S}^\adjoint\tilde{\ma{C}}_\mathcal{J}.
	\end{align}
	To do so, we propose a recurrence. \\
	\textit{Initialisation}. It is true for $n=1$, where $\mathcal{S}_1$ is reduced to $\{s_1\}$  and:
	\begin{align}
		\tilde{\ma{C}}_\mathcal{S}^{-1} = \frac{1}{\vec{\psi}_{s_1}^\adjoint\tilde{\ma{C}}_\mathcal{J}\vec{\psi}_{s_1}}
	\end{align}
	is a scalar and:
	\begin{align}
		\vec{f}_1\vec{f}_1^\adjoint = \frac{\vec{k}_1\vec{k}_1^\adjoint}{\vec{\psi}_{s_1}^\adjoint\vec{k}_1} = \frac{\tilde{\ma{C}}_\mathcal{J}\vec{\psi}_{s_1}\vec{\psi}_{s_1}^\adjoint\tilde{\ma{C}}_\mathcal{J}}{\vec{\psi}_{s_1}^\adjoint\tilde{\ma{C}}_\mathcal{J}\vec{\psi}_{s_1}} = \tilde{\ma{C}}_\mathcal{J} \vec{\psi}_{s_1}\tilde{\ma{C}}_\mathcal{S}^{-1} \vec{\psi}_{s_1}^\adjoint\tilde{\ma{C}}_\mathcal{J}.
	\end{align}
	\textit{Hypothesis}. We assume that Eq.~\eqref{eq:to_proove} is true at iteration $n-1$.\\%, \ie :\vspace{-0.2cm}
	%\begin{align}
	% \label{eq:recbis}
	%\forall i,j \quad \quad  \sum_{l=1}^{n-1} f_l(i)f_l(j) = \ma{K}_{\mathcal{S}_{n-1},i}^\adjoint \ma{K}_{\mathcal{S}_{n-1}}^{-1} %\ma{K}_{\mathcal{S}_{n-1},j}.\vspace{-0.3cm}
	% \end{align}
	\textit{Recurrence}. Let us show it is also true at iteration $n$. Using Woodbury's identity on $\tilde{\ma{C}}_\mathcal{S}^{-1}$, we show that:
	\begin{align}
	\tilde{\ma{C}}_\mathcal{J}\ma{\Psi}_\mathcal{S}\tilde{\ma{C}}_\mathcal{S}^{-1} \ma{\Psi}_\mathcal{S}^\adjoint\tilde{\ma{C}}_\mathcal{J}&=\tilde{\ma{C}}_\mathcal{J}\ma{\Psi}_{\mathcal{S}-1}\tilde{\ma{C}}_{\mathcal{S}-1}^{-1} \ma{\Psi}_{\mathcal{S}-1}^\adjoint\tilde{\ma{C}}_\mathcal{J} \\
	&+ \tilde{\ma{C}}_\mathcal{J}\frac{\vec{\psi}_{s_n}\vec{\psi}_{s_n}^\adjoint - \ma{\Psi}_{\mathcal{S}-1}\tilde{\ma{C}}_{\mathcal{S}-1}^{-1}\vec{u}\vec{\psi}_{s_n}^\adjoint-\vec{\psi}_{s_n} \vec{u}^\adjoint\tilde{\ma{C}}_{\mathcal{S}-1}^{-1}\ma{\Psi}_{\mathcal{S}-1}+\ma{\Psi}_{\mathcal{S}-1}\tilde{\ma{C}}_{\mathcal{S}-1}^{-1}\vec{u}\vec{u}^\adjoint\tilde{\ma{C}}_{\mathcal{S}-1}^{-1}\ma{\Psi}_{\mathcal{S}-1}^\adjoint}{z}\tilde{\ma{C}}_\mathcal{J},
	\end{align}
	where $\vec{u} = \ma{\Psi}_{\mathcal{S}-1}^\adjoint \tilde{\ma{C}}_\mathcal{J}\vec{\psi}_{s_n}$ and $z=\vec{\psi}_{s_n}^\adjoint \tilde{\ma{C}}_\mathcal{J}\vec{\psi}_{s_n}-\vec{u}^\adjoint \tilde{\ma{C}}_{\mathcal{S}-1}^{-1}\vec{u}$. 
	Replacing $\tilde{\ma{C}}_\mathcal{J}\ma{\Psi}_{\mathcal{S}-1}\tilde{\ma{C}}_{\mathcal{S}-1}^{-1} \ma{\Psi}_{\mathcal{S}-1}^\adjoint\tilde{\ma{C}}_\mathcal{J}$ by $\sum_{l=1}^{n-1} \vec{f}_l\vec{f}_l^\adjoint$ thanks to the hypothesis, the proof boils down to showing that:
	%    \begin{align}
	%   \ma{K}_{\mathcal{S},i}^\adjoint \ma{K}_{\mathcal{S},\mathcal{S}}^{-1} \ma{K}_{\mathcal{S},j} &= \sum_{l=1}^{n-1} f_l(i)f_l(j) + \frac{z_n(i)z_n(j)}{z_n(s_n)}. 
	% \end{align}
	% Il nous reste donc à montrer que :
	\begin{align}
	\label{eq:reste_a_montrer}
	\vec{f}_n\vec{f}_n^\adjoint=\tilde{\ma{C}}_\mathcal{J}\frac{\vec{\psi}_{s_n}\vec{\psi}_{s_n}^\adjoint - \ma{\Psi}_{\mathcal{S}-1}\tilde{\ma{C}}_{\mathcal{S}-1}^{-1}\vec{u}\vec{\psi}_{s_n}^\adjoint-\vec{\psi}_{s_n} \vec{u}^\adjoint\tilde{\ma{C}}_{\mathcal{S}-1}^{-1}\ma{\Psi}_{\mathcal{S}-1}+\ma{\Psi}_{\mathcal{S}-1}\tilde{\ma{C}}_{\mathcal{S}-1}^{-1}\vec{u}\vec{u}^\adjoint\tilde{\ma{C}}_{\mathcal{S}-1}^{-1}\ma{\Psi}_{\mathcal{S}-1}^\adjoint}{z}\tilde{\ma{C}}_\mathcal{J}
	\end{align}
	By construction of Algorithm~\ref{alg:sampling_r-DPP_bis_dual_efficient}, $\vec{f}_n\vec{f}_n^\adjoint$ reads :
	\begin{align}
	\label{eq:f}
	\vec{f}_n\vec{f}_n^\adjoint = \frac{(\tilde{\ma{C}}_\mathcal{J}\vec{\psi}_{s_n}-\sum_{l=1}^{n-1}\vec{f}_l\vec{f}_l^\adjoint\vec{\psi}_{s_n})(\vec{\psi}_{s_n}^\adjoint\tilde{\ma{C}}_\mathcal{J}-\vec{\psi}_{s_n}^\adjoint\sum_{l=1}^{n-1}\vec{f}_l\vec{f}_l^\adjoint)}{\vec{\psi}_{s_n}^\adjoint \tilde{\ma{C}}_\mathcal{J}\vec{\psi}_{s_n}-\vec{\psi}_{s_n}^\adjoint \sum_{l=1}^{n-1}\vec{f}_l\vec{f}_l^\adjoint \vec{\psi}_{s_n}} 
	\end{align}
	Using a second time the hypothesis to replace $\sum_{l=1}^{n-1}\vec{f}_l\vec{f}_l^\adjoint$ by  $\tilde{\ma{C}}_\mathcal{J} \ma{\Psi}_{\mathcal{S}-1}\tilde{\ma{C}}_{\mathcal{S}-1}^{-1} \ma{\Psi}_{\mathcal{S}-1}^\adjoint\tilde{\ma{C}}_\mathcal{J}$, we show Eq.~\eqref{eq:reste_a_montrer}, which ends the proof.
	%
	%
	%on a :
	% \begin{align}
	%\forall i\quad\quad f_{n}(i) = \frac{\ma{K}_{s_{n},i} - \ma{K}_{\bar{\mathcal{S}},s_n}^\adjoint \ma{K}_{\bar{\mathcal{S}},%\bar{\mathcal{S}}}^{-1}\ma{K}_{\bar{\mathcal{S}},i}}{\sqrt{\ma{K}_{s_{n},s_{n}} - \ma{K}_{\bar{\mathcal{S}},s_n}^\adjoint \ma{K}_{\bar{\mathcal{S}},%\bar{\mathcal{S}}}^{-1}\ma{K}_{\bar{\mathcal{S}},s_n}}}.
	%\end{align}
	%Si bien que :
\end{proof}

\section{ \ifels\else - \fi More}
Let us first discuss the following choice of kernel:
\begin{align}
\label{eq:K}
\ma{K} = \alpha\ma{L}(\ma{I}+\alpha\ma{L})^{-1},
\end{align}
with $\alpha=1/\max_{i} \sum_j \ma{L}_{ij}$ a scaling factor that depends on $s$. $\alpha\ma{L}$ is called the $L$-ensemble associated to $\ma{K}$. 

\begin{theorem}
	Sampling a DPP from kernel $\ma{K}$ as in Eq.~\eqref{eq:K} provides an expected number of samples verifying:
	\begin{align*}
	\frac{\alpha N}{2}\leq \mu\leq \alpha N.
	\end{align*}
	Also, such samples form a $\epsilon$-coreset with probability at least $1-\delta$ provided that $\alpha$ (and thus $s$) is set such that:
	\begin{align}
	\label{eq:thm_K}
	\frac{\alpha^2}{1+\alpha}\geq \frac{32\sigma_\text{max}^2}{\epsilon^2\sigma_\text{min}} kd(\epsilon+4\mathfrak{S}) \log{\frac{60r^2}{\delta\epsilon\langle f\rangle_\text{opt}}}.
	\end{align}
\end{theorem}

\begin{proof}
	Let us write $\lambda'_i=\alpha\lambda_i$. As $\alpha=1/\max_{i} \sum_j \ma{L}_{ij}$, we have:
	\begin{align*}
	\forall i, \qquad 0\leq\lambda'_i\leq\lambda'_N\leq 1.
	\end{align*}
	The following is always verified:
	\begin{align*}
	\forall\lambda'\in[0,1]\qquad \frac{\lambda'}{2}\leq\frac{\lambda'}{1+\lambda'}\leq \frac{1}{4}(1+\lambda'),
	\end{align*}
	such that:
	\begin{align*}
	\pi_i = \ma{K}_{ii}=\sum_k \frac{\lambda_k'}{1+\lambda_k'} \fou_k(i)^2
	\end{align*}
	verifies:
	\begin{align*}
	\frac{\alpha}{2} = \frac{\alpha}{2}\ma{L}_{ii}=\sum_k \frac{\lambda_k'}{2} \fou_k^2(i)\leq \pi_i \leq \sum_k \frac{1}{4}(1+\lambda') \fou_k^2(i)=\frac{1}{4}(1+\alpha).
	\end{align*}
	Writing $\beta=\frac{\alpha}{2\sigma_\text{max}}$, we have:
	\begin{align*}
	\forall i, \qquad \beta\sigma_i\leq \frac{\alpha}{2}\leq \pi_i.
	\end{align*}
	And writing $\gamma=\frac{1+\alpha}{\alpha}\frac{\sigma_\text{max}}{2\sigma_\text{min}}$, we have:
	\begin{align*}
	\forall i, \qquad \pi_i\leq \frac{1}{4}(1+\alpha) \leq \beta\gamma\sigma_i. 
	\end{align*}
	Moreover, as $0\leq\alpha\leq1$, we have that $\beta\leq\frac{1}{\sigma_\text{max}}$ and $\gamma\geq 1$ such that we verify condition~\eqref{eq:condition_1} of Corollary~\eqref{corollary:DPP_kmeans}.  
	Therefore, sampling from $\ma{K}$ provides a $\epsilon$-coreset if condition~\eqref{eq:condition_2} is also verified:
	\begin{align*}
	\qquad 	\frac{\beta}{\gamma}\geq\frac{32}{\epsilon^2} kd(\epsilon+4\mathfrak{S}) \log{\frac{60r^2}{\delta\epsilon\langle f\rangle_\text{opt}}},
	\end{align*}
	which may be rewritten as Eq.~\eqref{eq:thm_K}. 
\end{proof}
